# Supplementary material for: Homogeneously derived transit timings for 17 exoplanets and reassessed TTV trends for WASP-12 and WASP-4
Source: arXiv:1908.04505 source file (2019-08-13)
Supplement: Supplementary file 1 [file ttv_supplement.pdf]

MNRAS 000, 1–17 (2019) Preprint 12 August 2019 Compiled using MNRAS LaTeX style file v3.0

# Homogeneously derived transit timings for 17 exoplanets and reassessed TTV trends for WASP-12 and WASP-4

R.V. Baluev et al.

12 August 2019

**ABSTRACT**
This file contains an online-only supplementing material including the full set of full-sized figures and tables.

## 1 FULL SET OF FIGURES

See below, Fig. 1, 10, 11, 12 represent a full-size version of the figures from the main text. The other figures are presented only here.

© 2019 The Authors

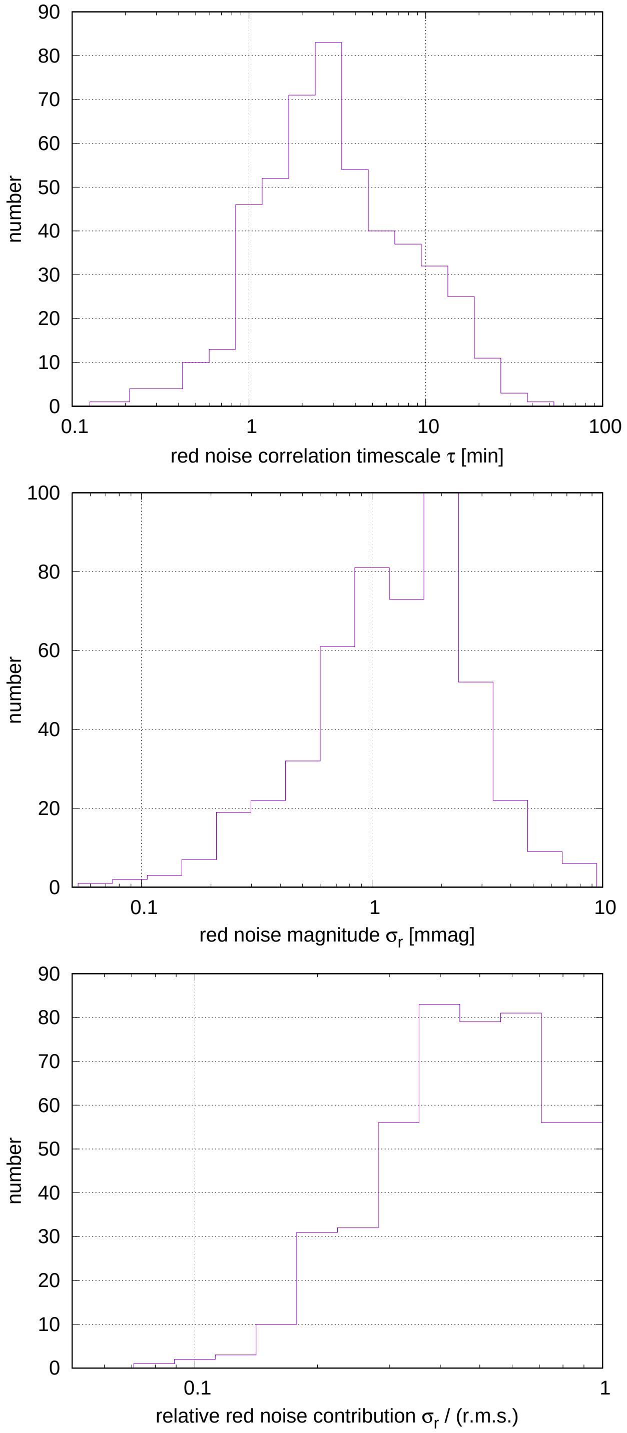


**Figure 1.** Histograms of the estimated photometric red noise parameters, $\tau$ and $\sigma_r$, and of the relative red noise contribution in the total r.m.s. We used only those estimations of $\tau$ and $\sigma_r$ on Stage 4 that exceeded their respective uncertainty.

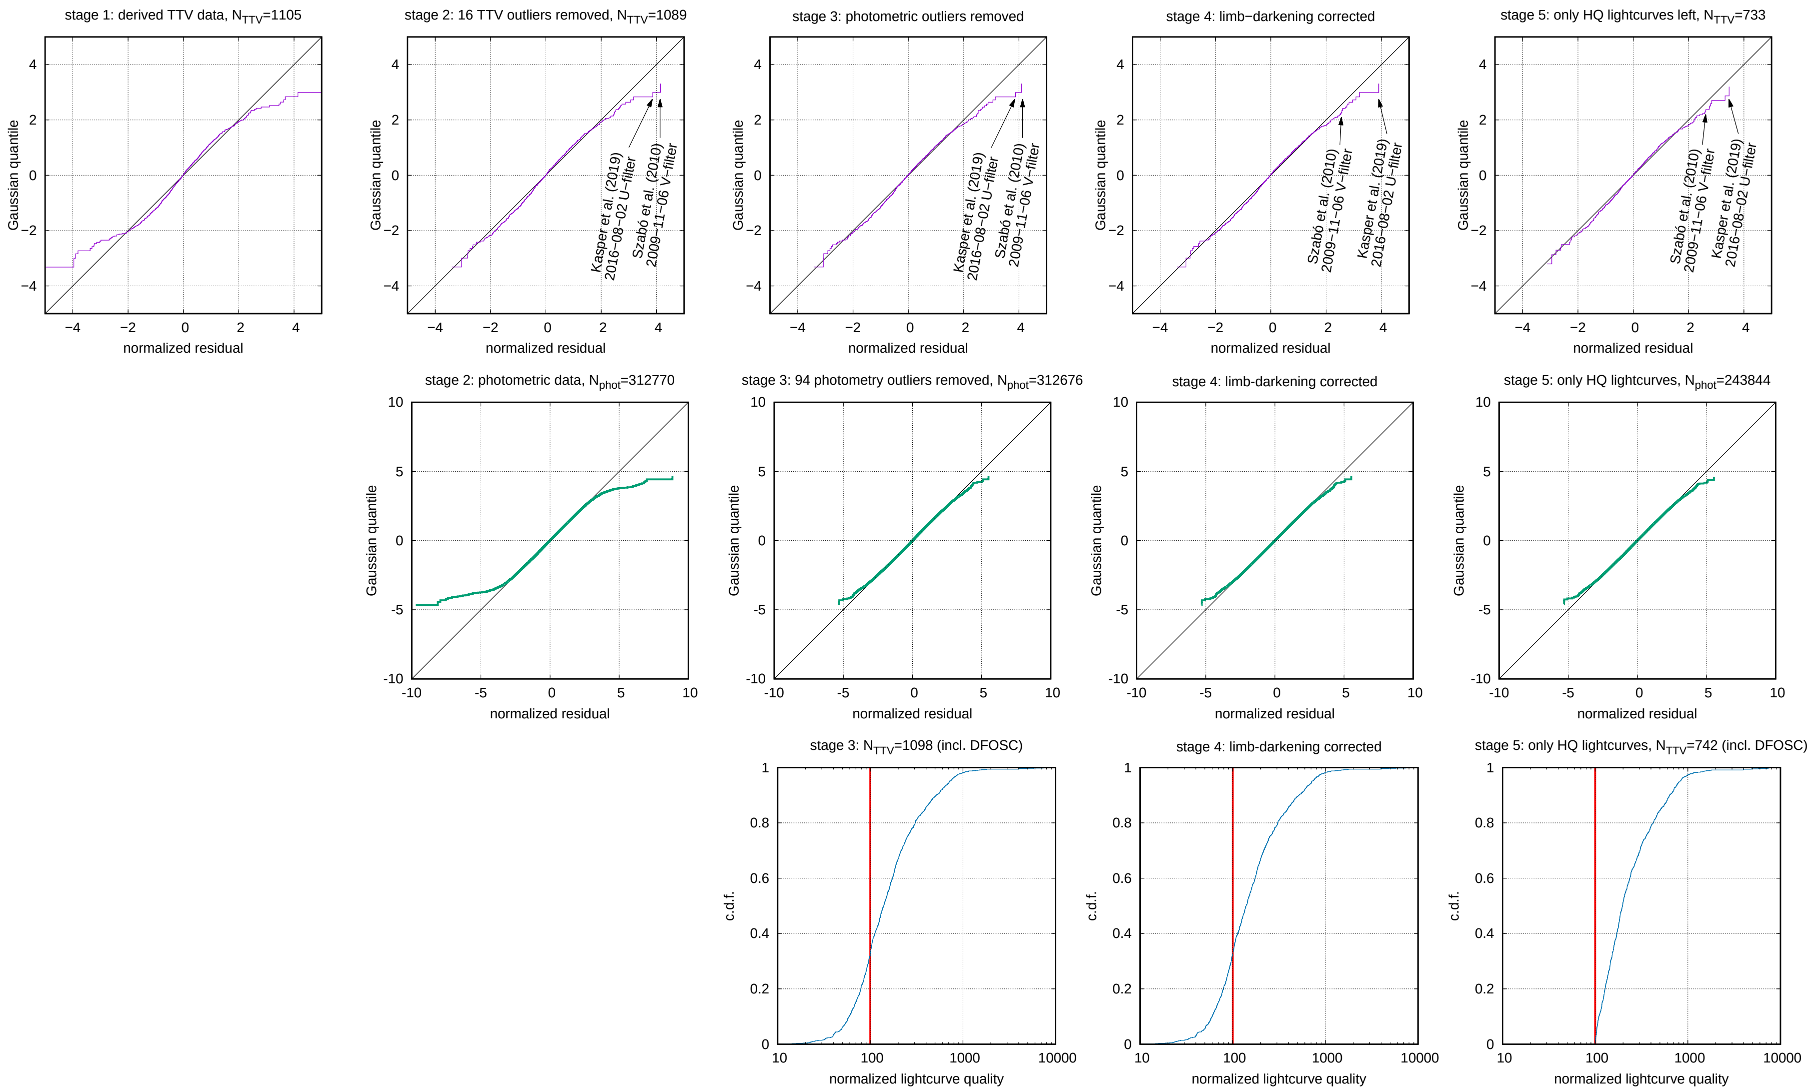


**Figure 2.** Clearing outliers and verifying the Gaussianity of the data. Top row: QQ plot for TTV residuals, middle: QQ plot for photometric residuals, bottom: CDF plot for the lightcurve quality characteristic. Columns correspond to different processing stages: (i) initial fit, (ii) removing TTV outliers (bad lightcurves), (iii) removing photometric outliers in individual lightcurves, (iv) setting semi-empirical limb-darkening coefficients for lightcurves that could not constrain limb-darkening well, (v) removing about 1/3 of the low-quality lightcurves.

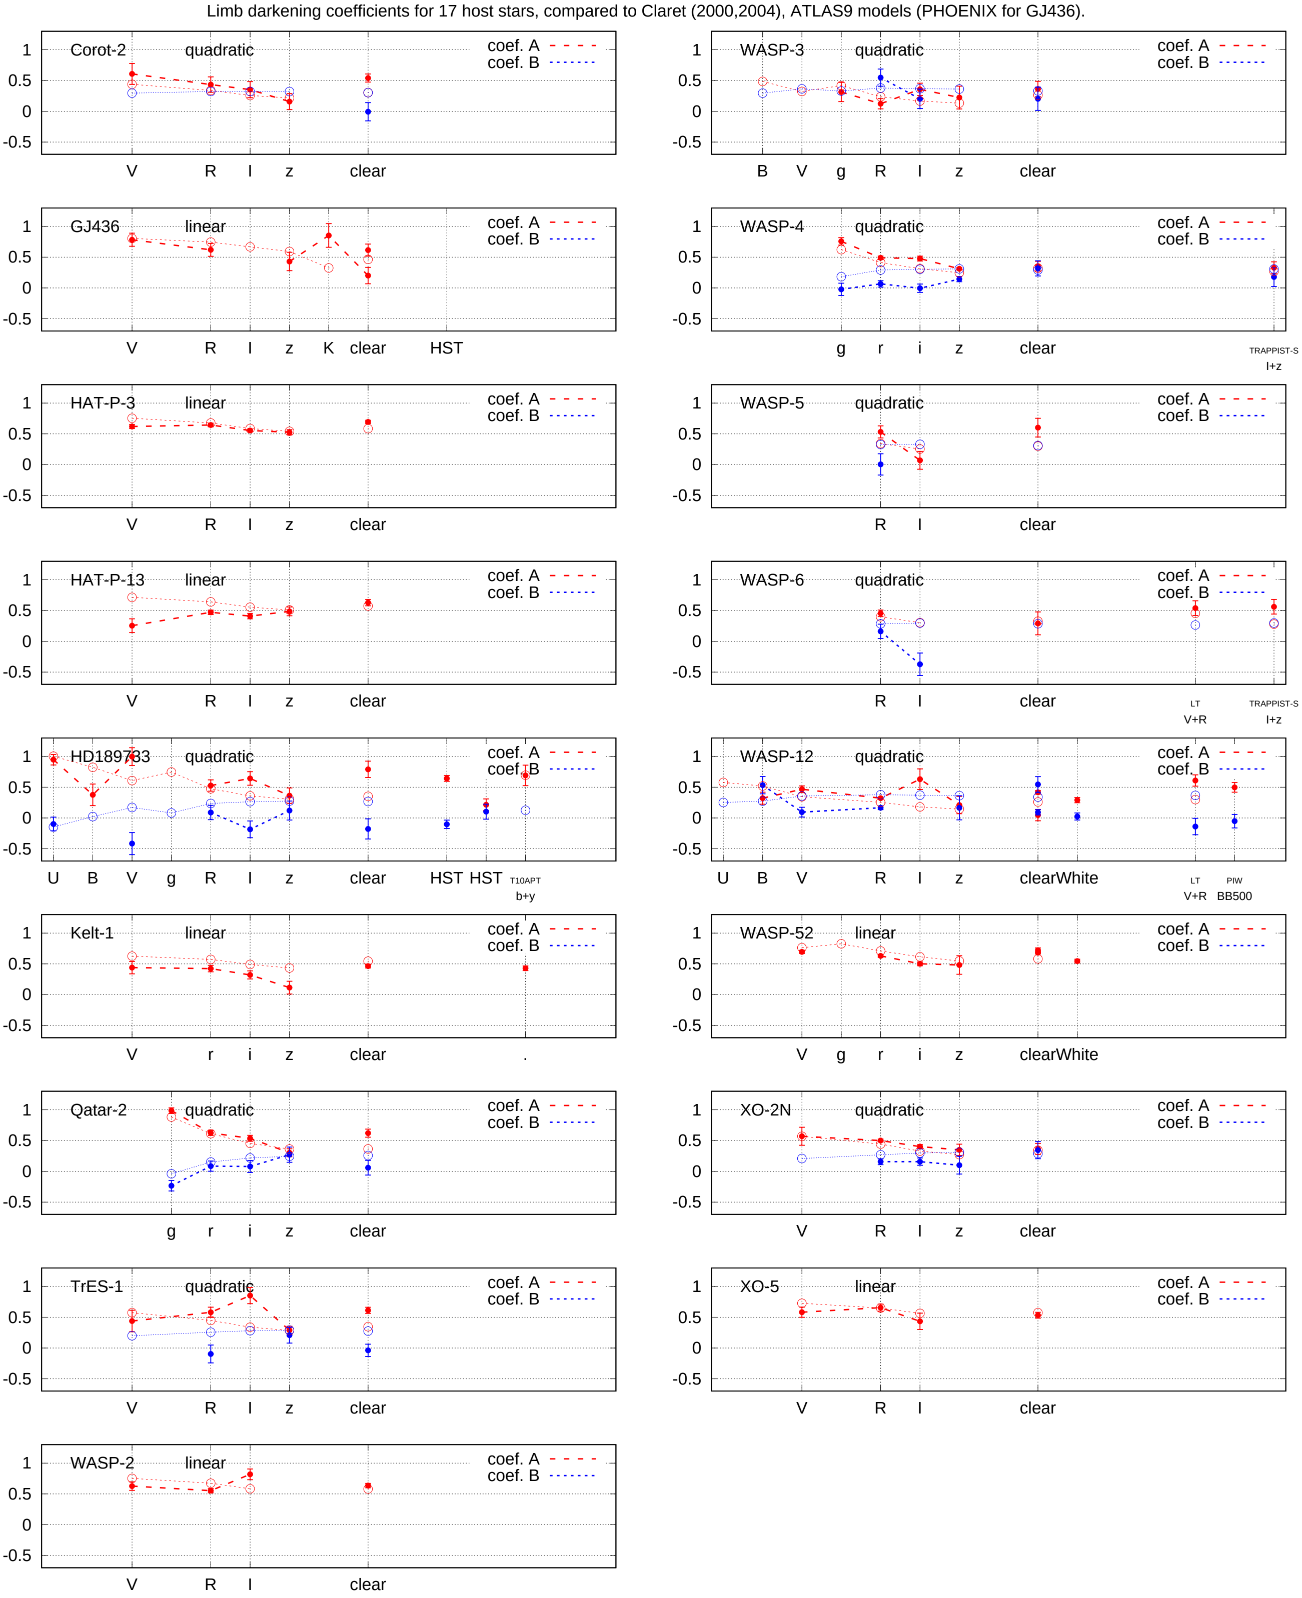


**Figure 3.** Empirical and theoretical limb darkening coefficients for our 16 targets, depending on the spectral filter. Points with error bars show the observed (fitted) values, and open circles label the theoretical values based on (Claret 2000, 2004). Too rough empirical estimations with an uncertainty above 0.2 are not shown. We show results either for the quadratic limb-darkening model, or for the linear one, if we had too few accurate coefficients for the quadratic law. The linear models are shown here only for a more informative demonstration, but the final processing was performed with a quadratic model for all the targets (see text).

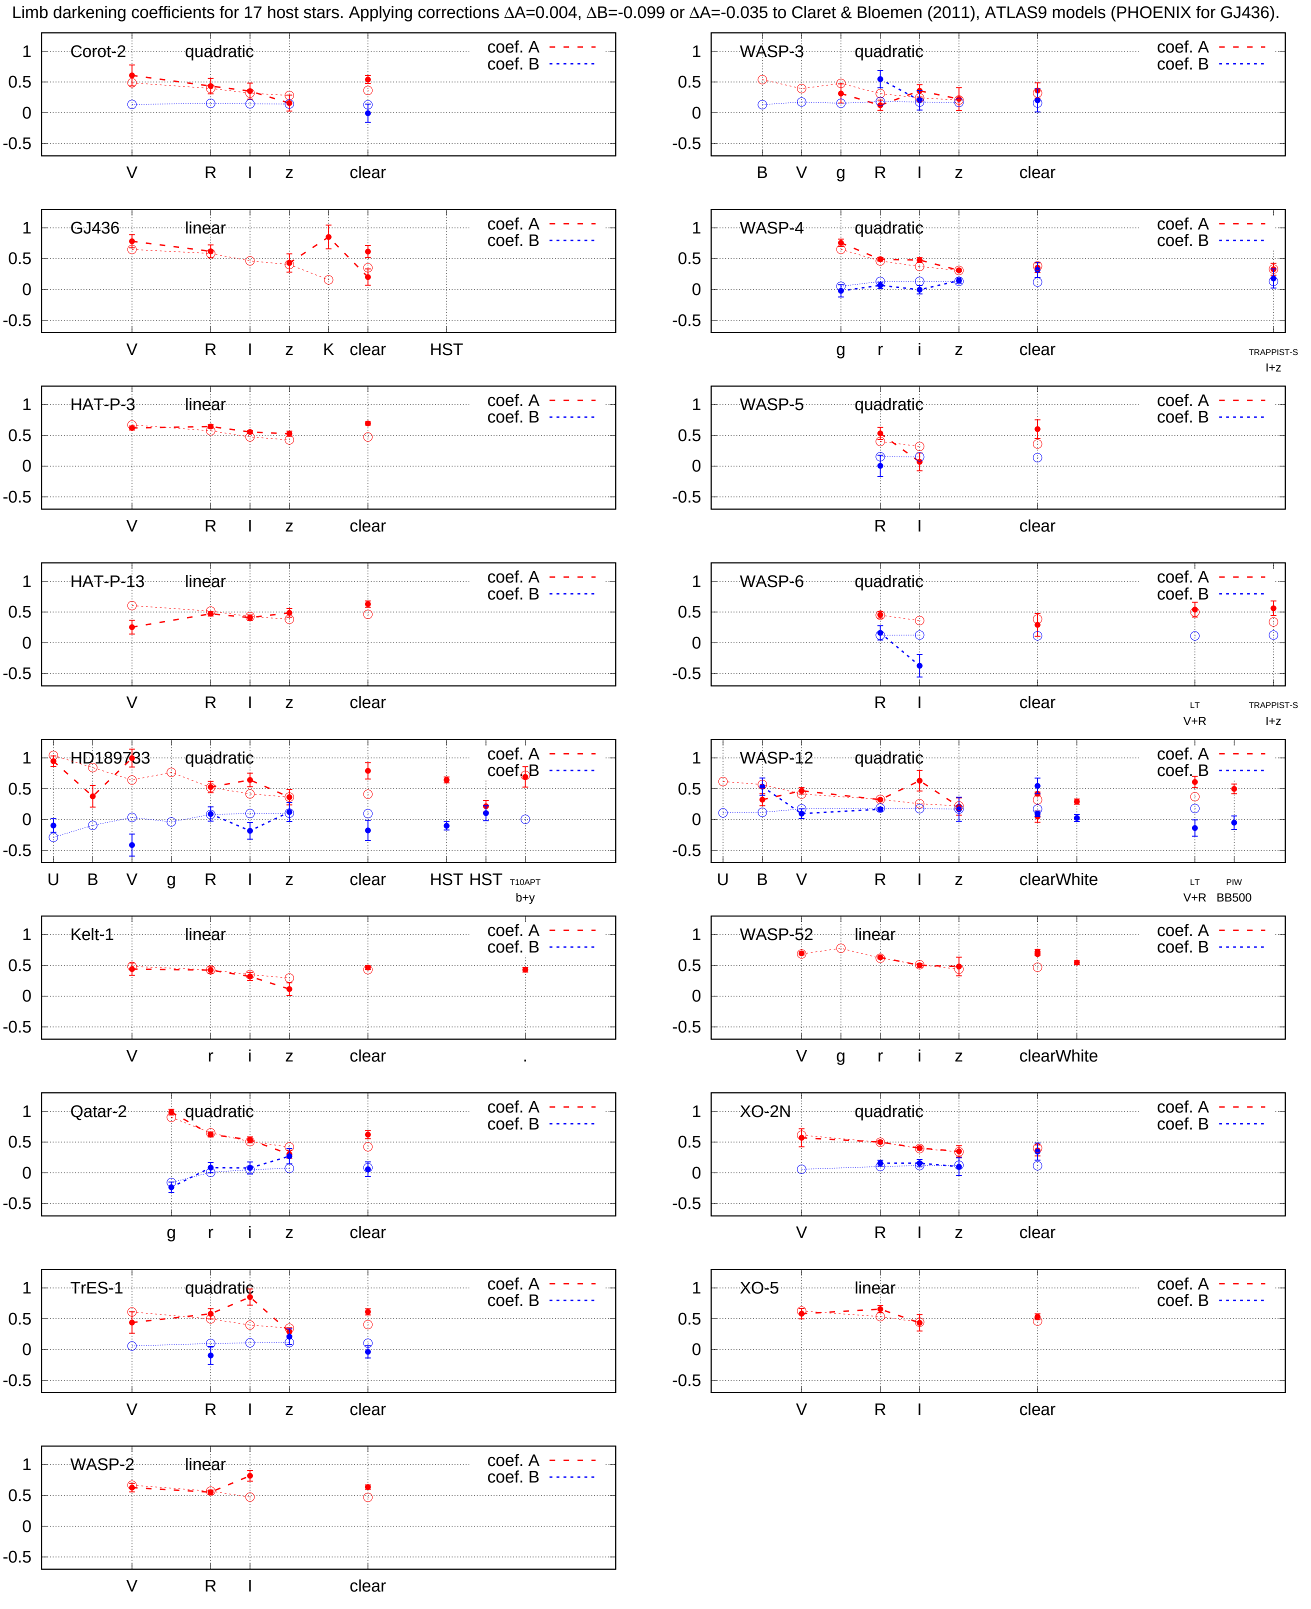


**Figure 4.** Same as Fig. 3, but for the newer theory models by Claret & Bloemen (2011), additionally corrected by the best-fitting offsets printed in the title. For the "clear" case we plot bolometric Claret (2000) models corrected by the biases determined on the basis of UBVGRIZK filters.

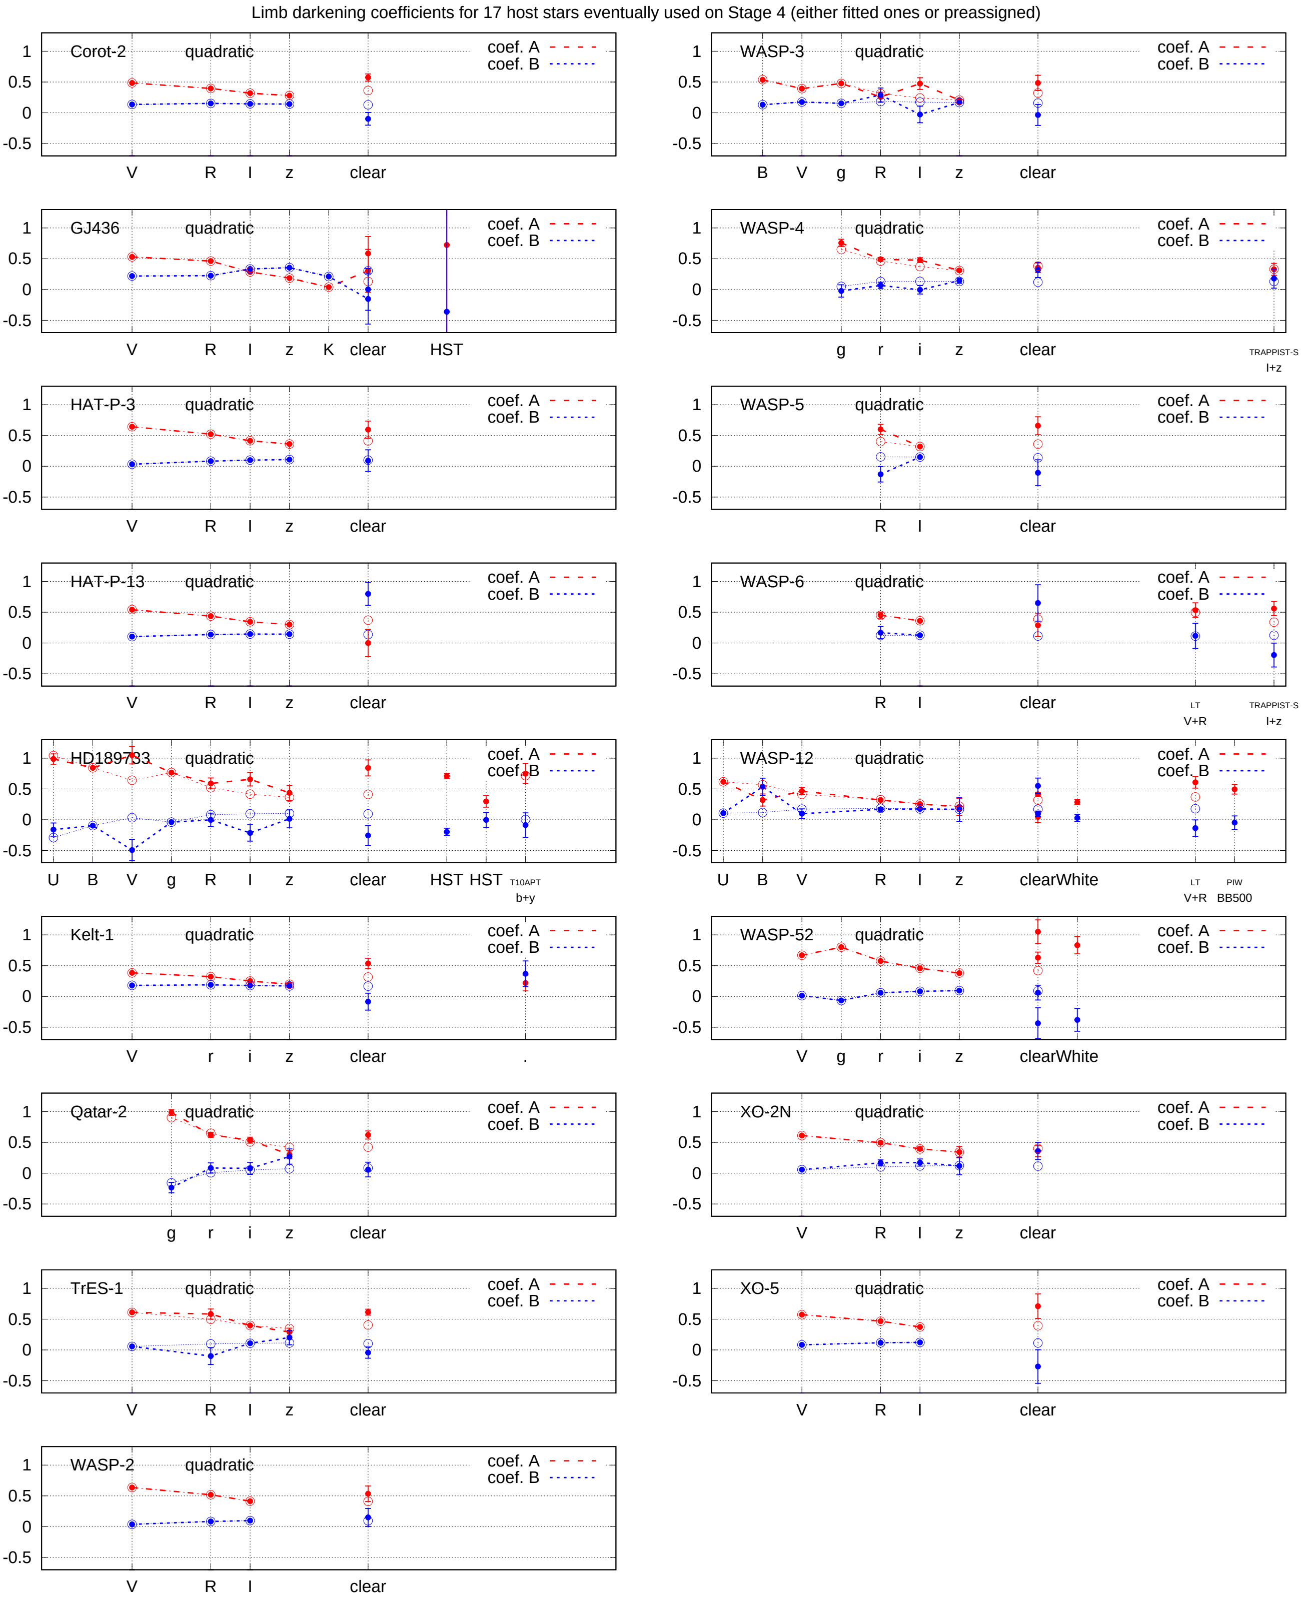


**Figure 5.** The limb-darkening coefficients used in our final fits. These are either the corrected theoretical coefficients by Claret & Bloemen (2011) or the best fitting values (if they had enough fitting accuracy). The corrected theoretical values are the same as those used in Fig. 4. Here we consider only the quadratic limb-darkening model for all the targets.

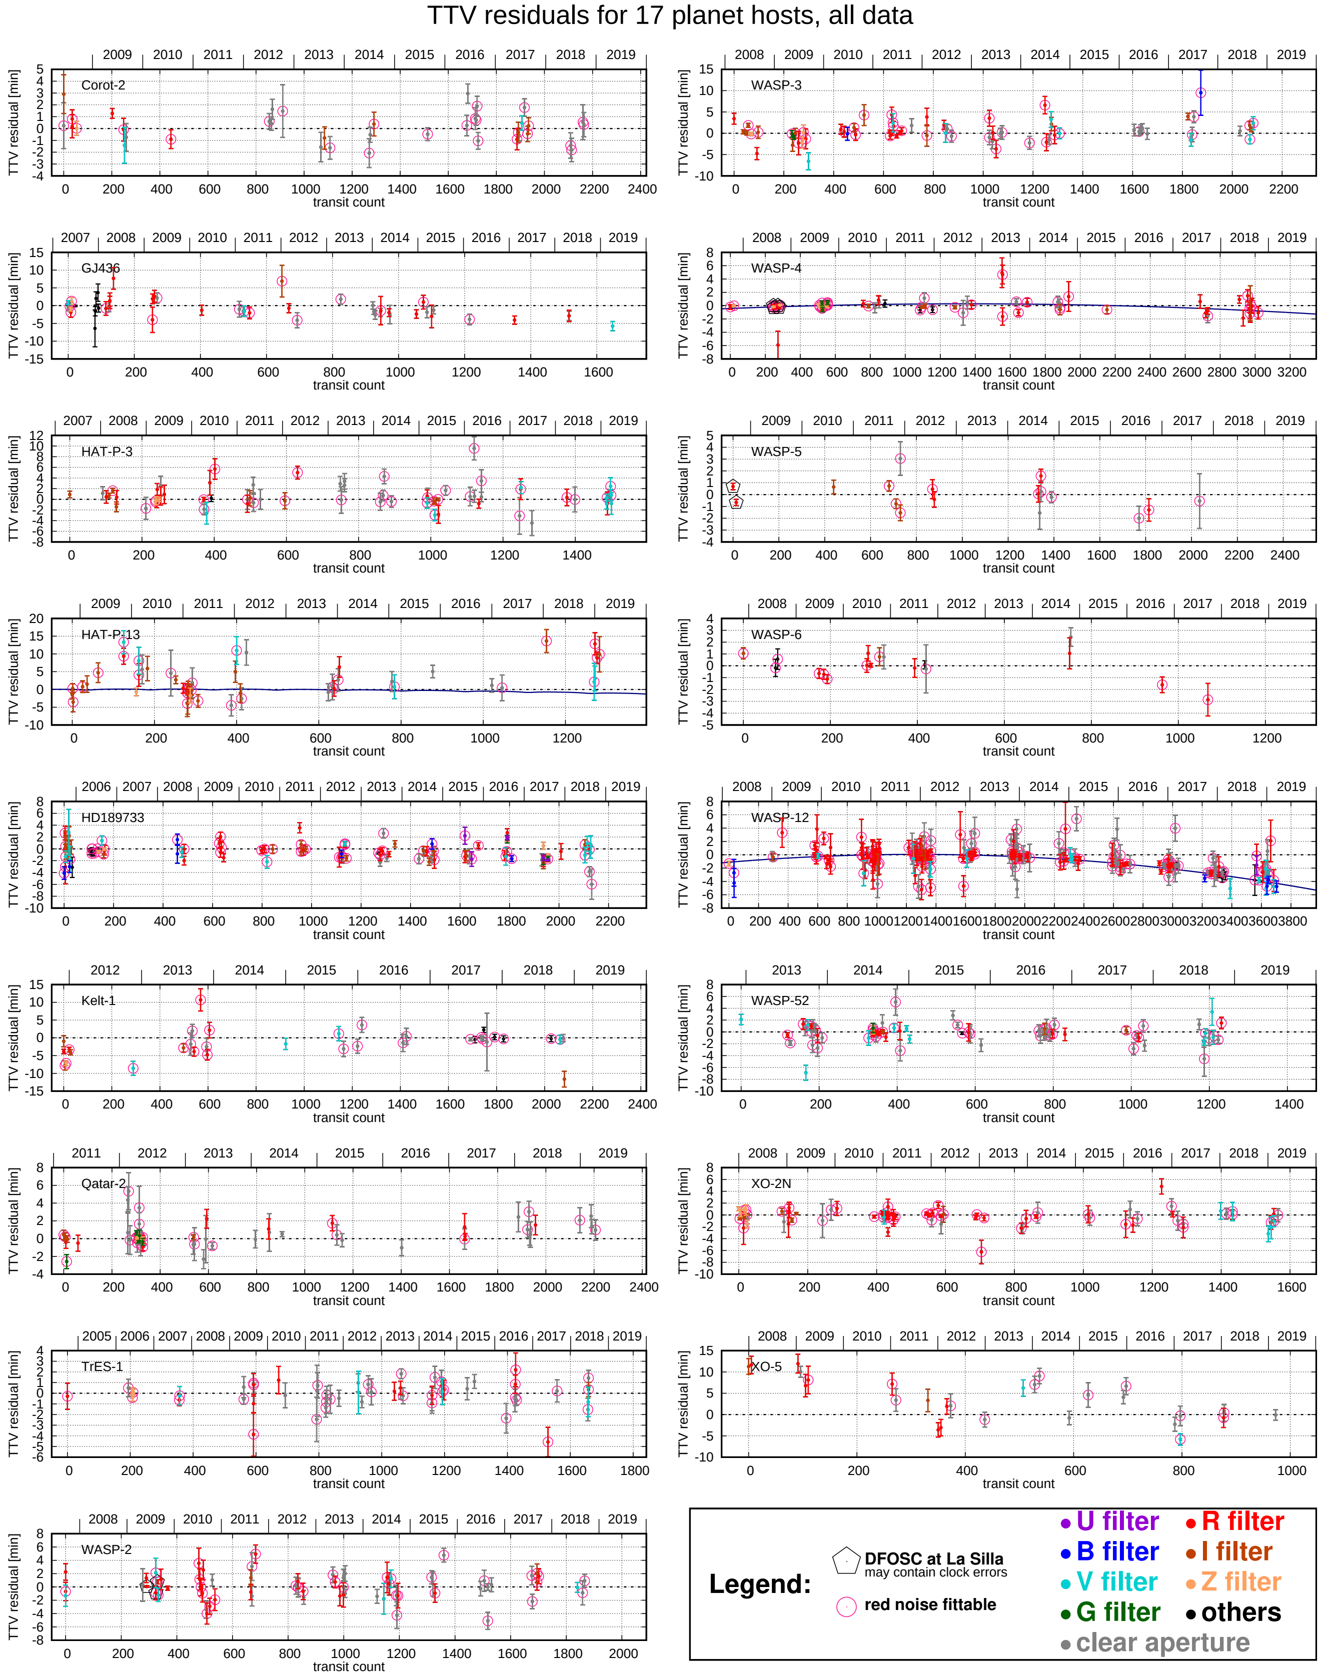


**Figure 6.** TTV residuals derived for the 17 targets by Stage 4 on the processing (after cleaning TTV and photometric outliers, and correcting the limb-darkening). The plots only show points with at most 2 min uncertainty. For WASP-12 we also plot the quadratic trend derived by (Patra et al. 2017). For WASP-4 we show the suspected trend from Bouma et al. (2019). For HAT-P-13 we also plot the expected Roemer effect curve induced by the second companion and by the radial acceleration term (derived in the main paper).

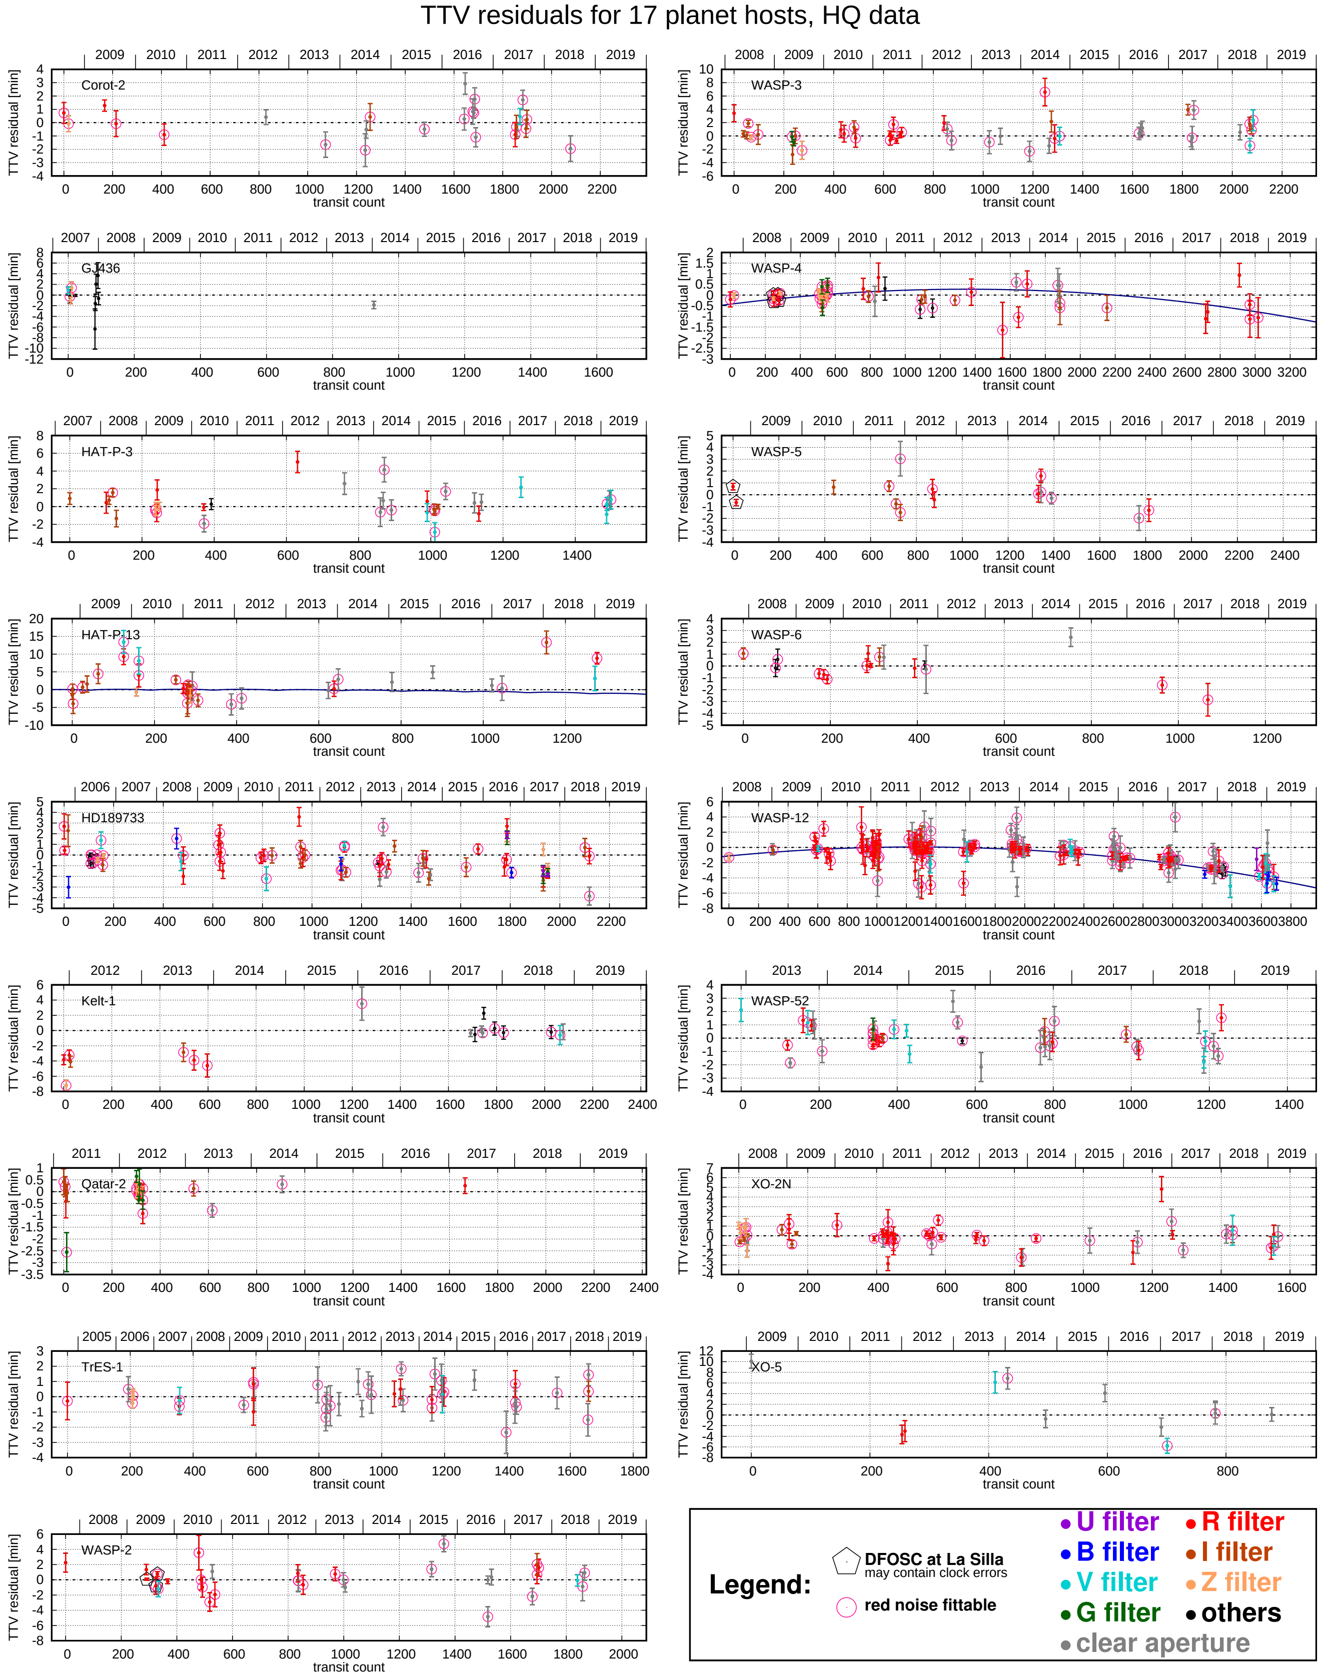


**Figure 7.** Same as Fig. 6, but for Stage 5 (when keeping only HQ lightcurves).

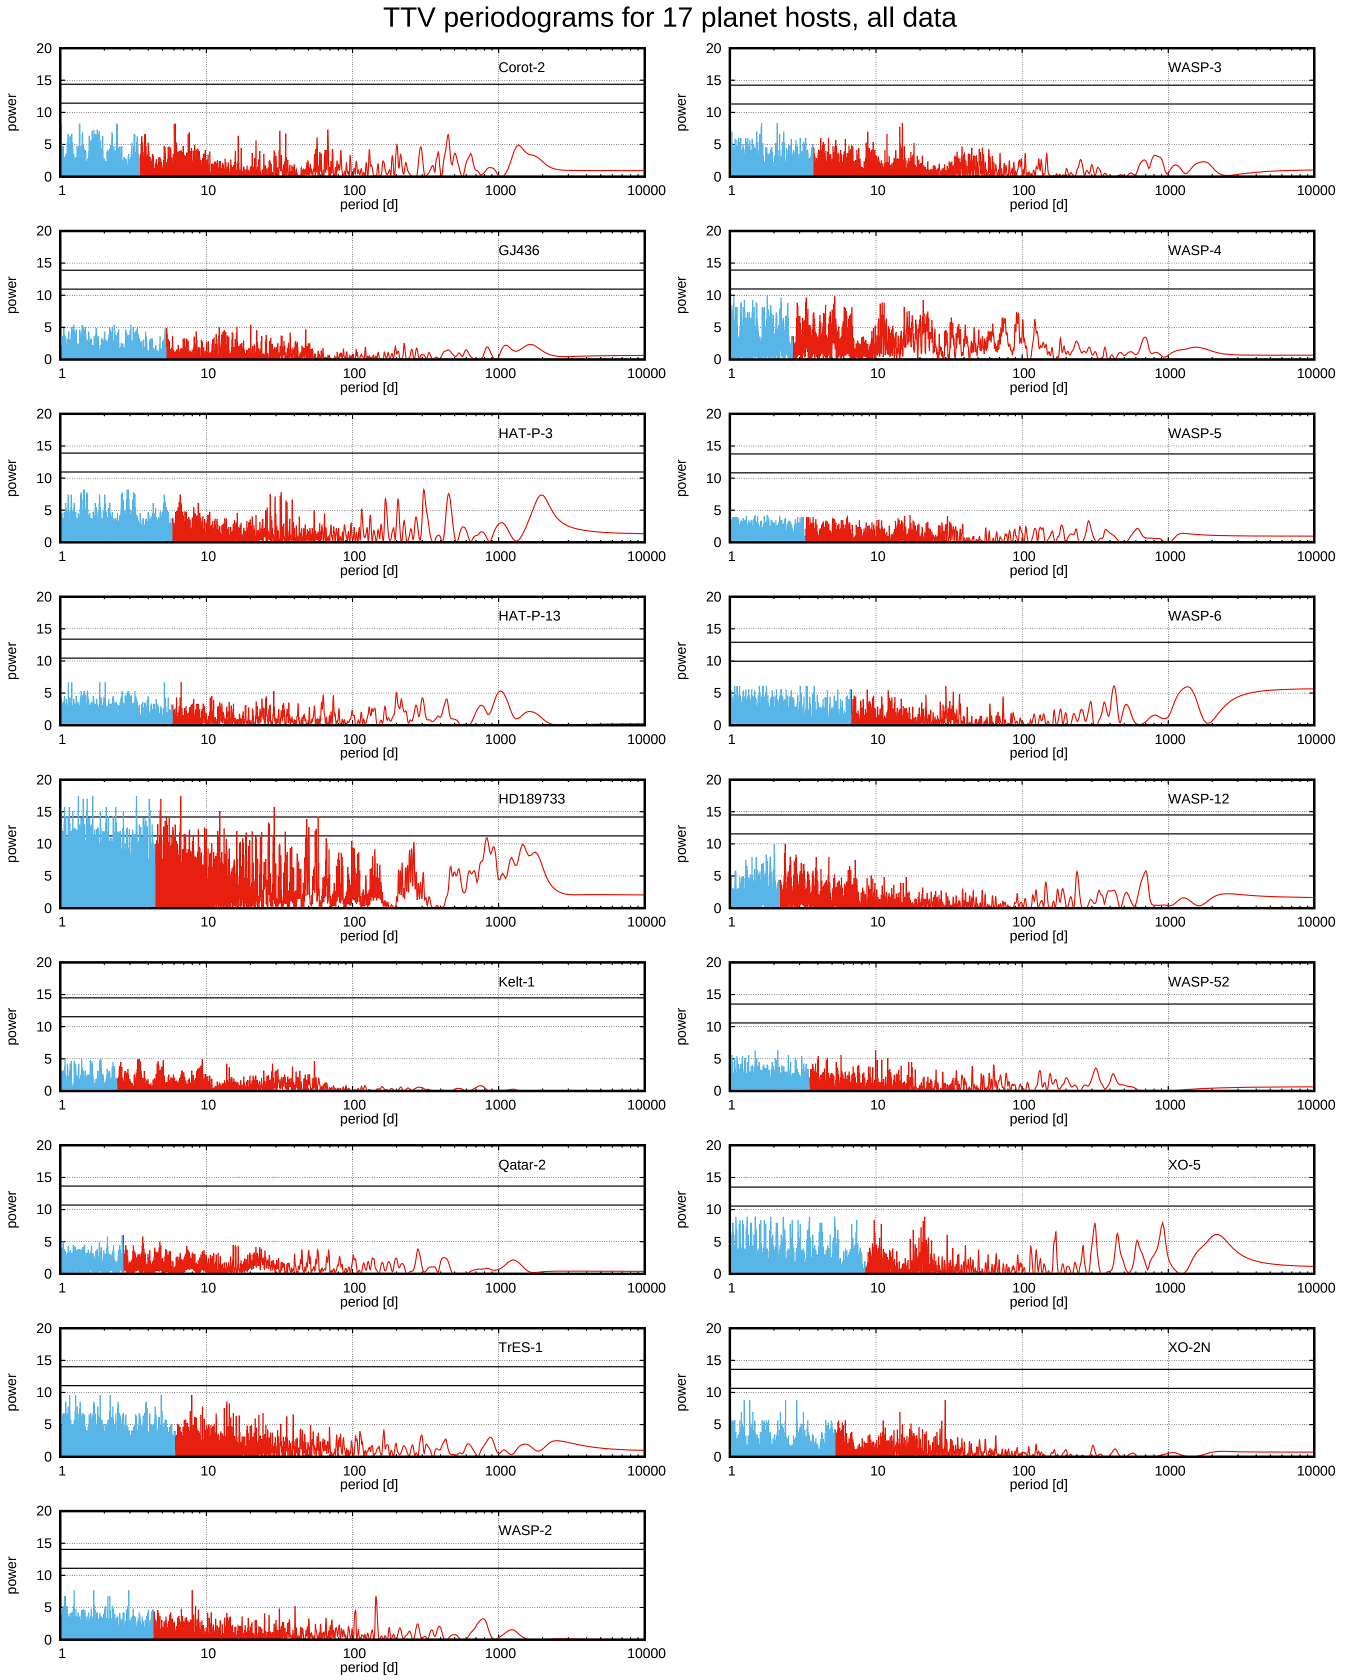


**Figure 8.** Periodograms of the derived TTV data (Stage 4, all data). Red is the primary Nyquist frequency range, blue is its continuation by periodogram symmetry and periodicity properties. Two horizontal lines label 2-sigma and 3-sigma significance levels determined from (Baluev 2008).

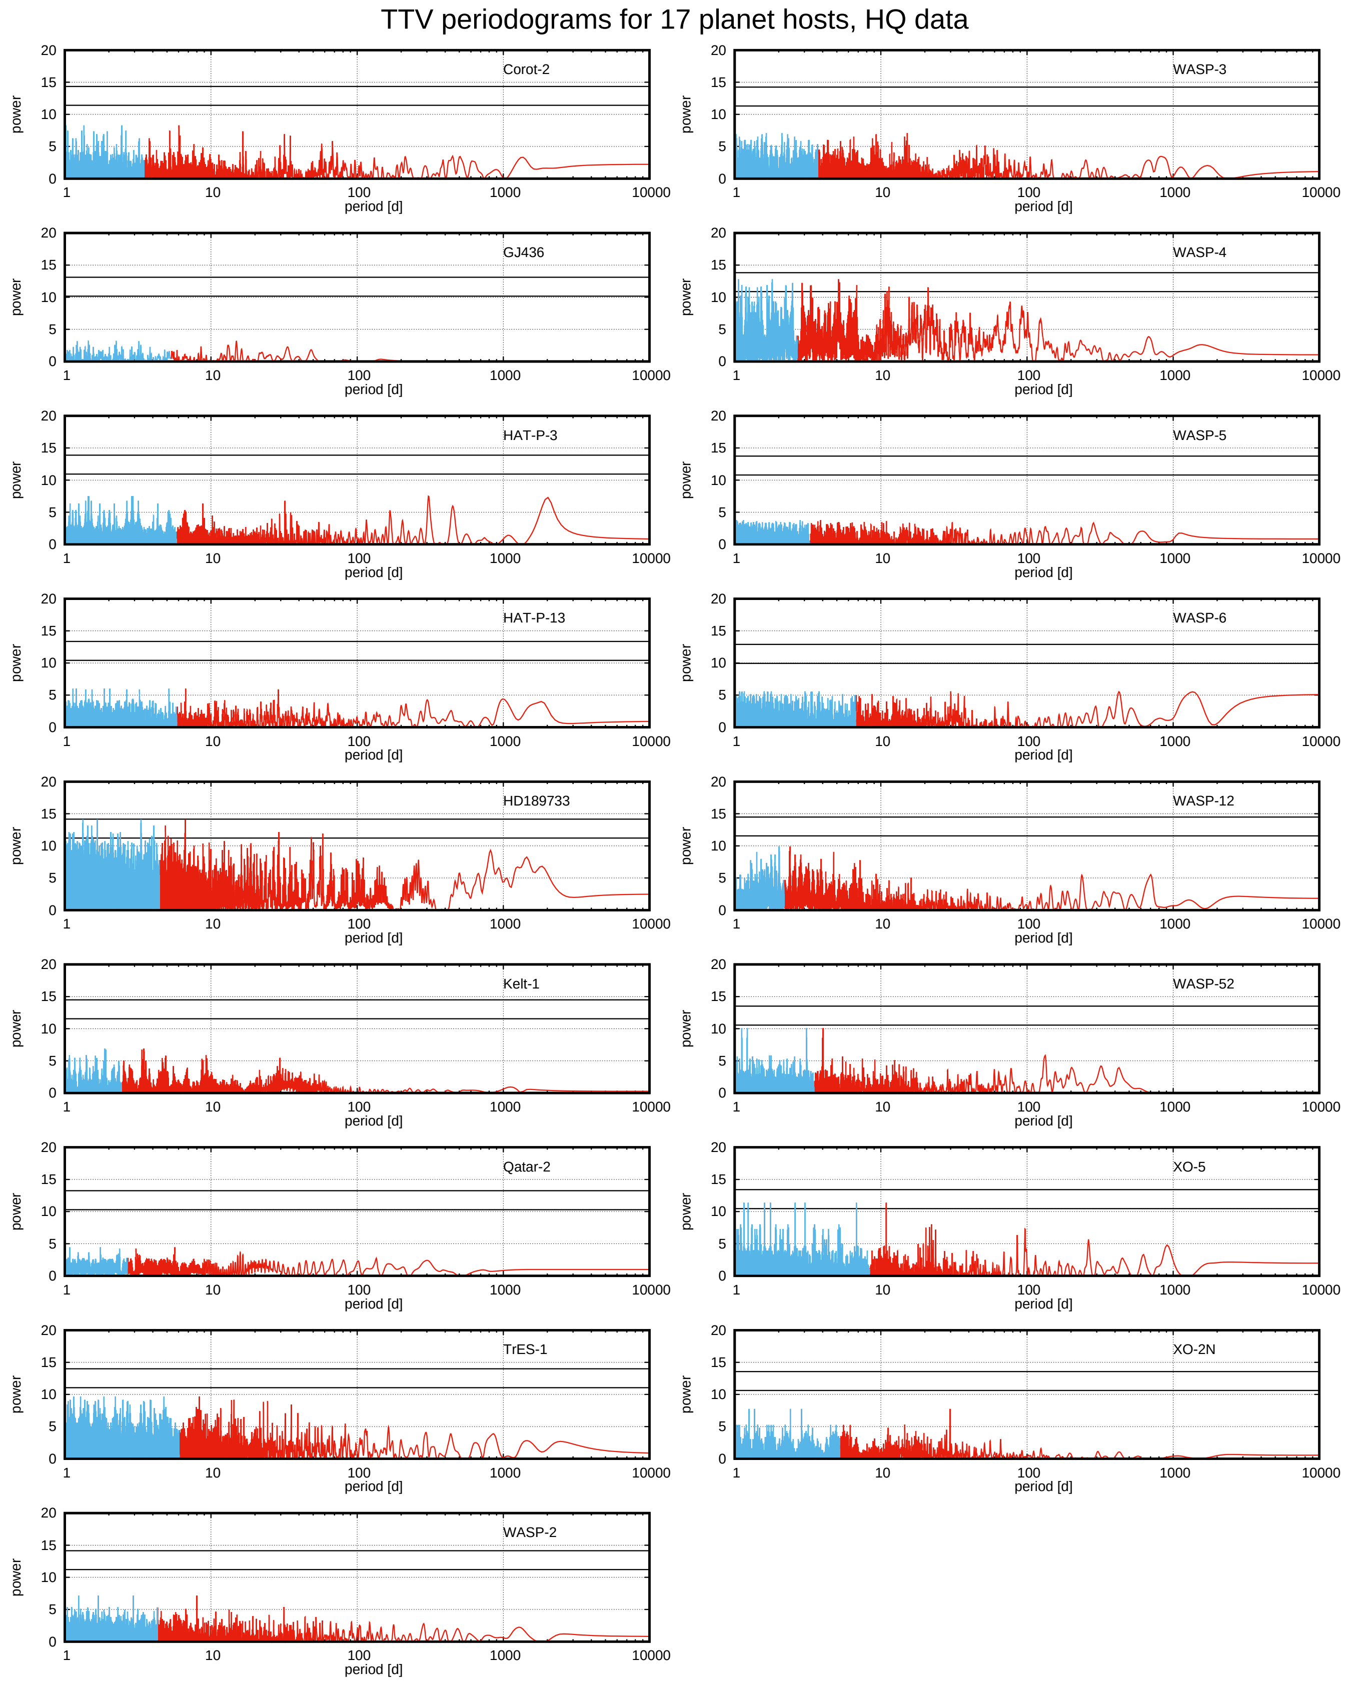


**Figure 9.** Same as Fig. 8, but for Stage 5 (HQ data only).

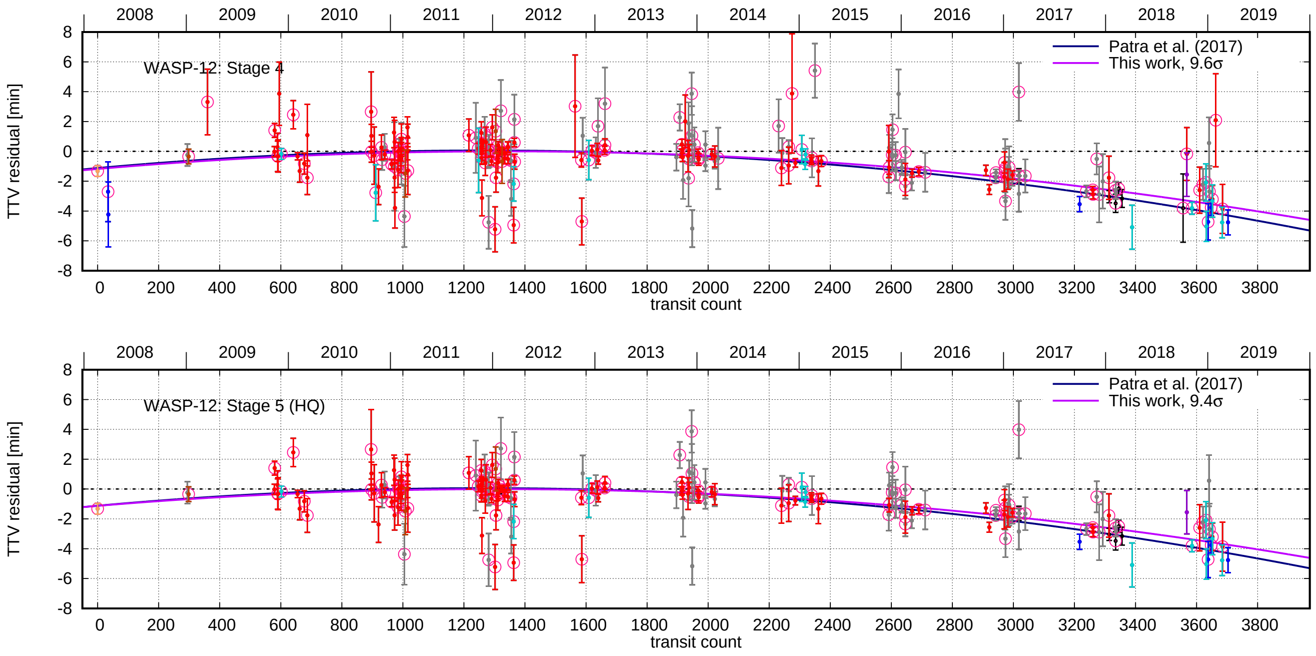


**Figure 10.** Transit times of WASP-12 derived in this work. Top panel is for all the TTV data (stage 4), bottom panel is for only HQ ones (stage 5). The models of the quadratic TTV trend are also plotted (for the multiplicative noise model).

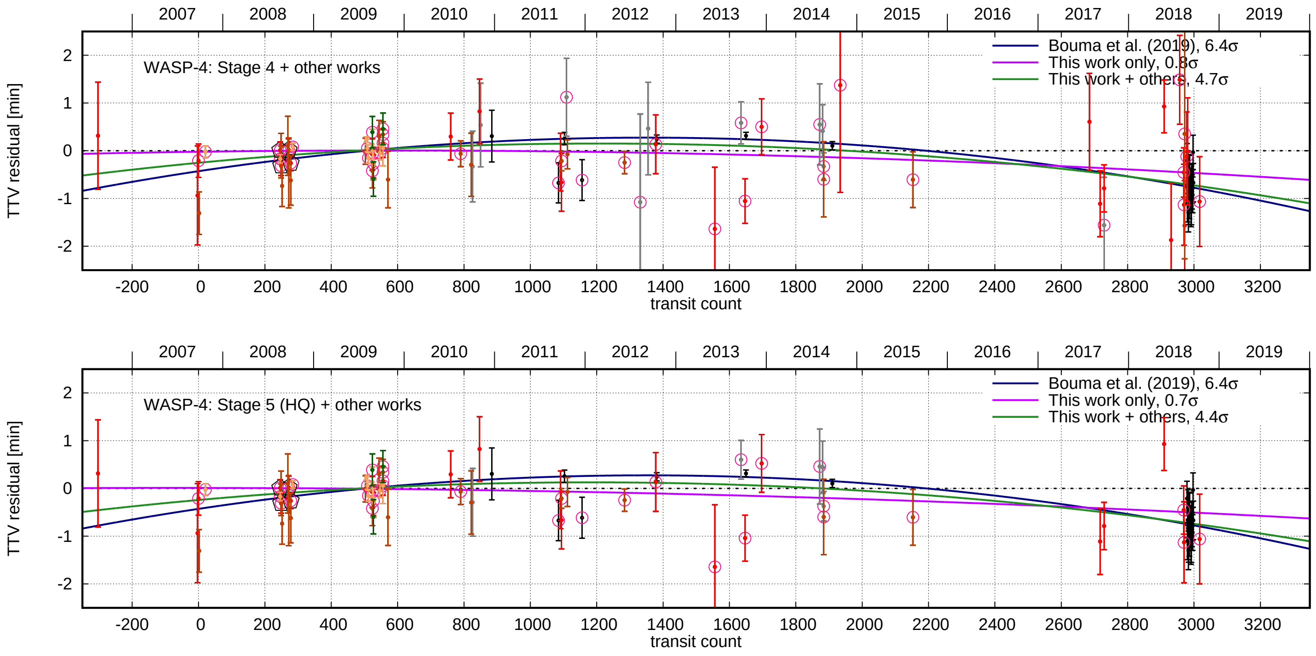


**Figure 11.** Transit times of WASP-4, including the homogeneous sample from this work (without DFOSC data possibly affected by clock errors), and the timing data published in literature without lightcurves. Top panel is for all the TTV data (Stage 4), bottom panel is for only HQ ones (Stage 5). Several models of the quadratic TTV trend are also plotted with the $\chi^2$-test trend significance labelled in the legend. Except for (Bouma et al. 2019), these trends correspond to the best fitting model involving the regularized noise, that softens the weights contrast, and assuming a simple merge of heterogeneous TTV data into a single time series.

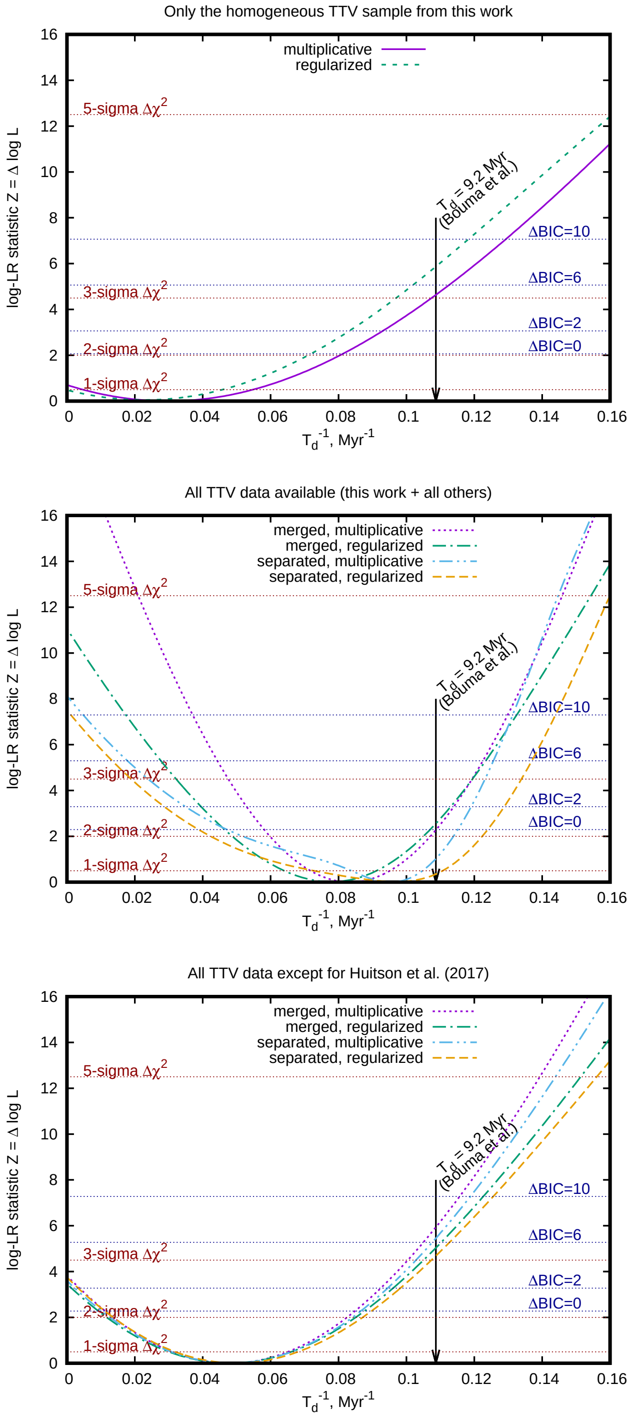


**Figure 12.** Logarithm of the likelihood ratio statistic for WASP-4, $Z(q)$, as a function of $q = T_{\mathrm{d}}^{-1}$. Three graphs correspond to different compilations of TTV data (homogeneous from this work / all / all but Huitson et al. (2017)). The curves within each graph correspond to different models of the TTV noise (merged/separated and multiplicative/regularized). In each graph a set of the significance threshold levels is also shown, corresponding to the frequentist $\chi^2$ test or to the Bayesian information criterion (BIC). See text for more details and a discussion.

## 2 FULL-SIZED TABLES

See below, Table 1 represents a full-font-size version of the table from the main text. The other tables also contain additional data.

**Table 1.** Fitted parameters of exoplanetary transit curves after Stages 4 and 5 processing.

| transiter host | total number of transits $N$ | Assuming fittable transit times: number of red-noised lightcurves[3] | aggregate quality[1] $\mathcal{Q}'_{\rm sum}$ | radii ratio $r = R_{\rm pl}/R_\star$ | half-duration $t_d/2$ [days] | impact par. $b$ | $\sqrt{\chi^2_{\rm TTV}}$ [2] | mid-times correl. MAD | mid-times correl. MAX | Fixing timings at a quadratic model[2]: ref. mid-time[5] $T_0$ [BJD$_{\rm TDB}-$ $-2450000$] | orbital period[5] $P$ [days] | quadr. trend[5] $dP/dn$ [$10^{-10}$day] |
|---|---|---|---|---|---|---|---|---|---|---|---|---|
| Corot-2 | 38 | 13 + 12 | 893 | 0.16524(93) | 0.04726(20) | 0.158(70) | 1.37 | 0.00034 | 0.006 | 7622.43669(11) | 1.74299767(36) | 2.6(5.1) |
| GJ436[4] | 47 | 8 + 7 | 857 | 0.0847(10) | 0.02108(21) | 0.8612(66) | 1.10 | 0.0022 | 0.66 | 4439.41624(10) | 2.64389938(67) | −28(12) |
| HAT-P-13 | 51 | 19 + 12 | 1470 | 0.08826(78) | 0.06919(38) | 0.7500(77) | 1.55 | 0.0011 | 0.036 | 5476.91220(19) | 2.9162394(14) | 92(33) |
| HAT-P-3 | 66 | 16 + 16 | 1400 | 0.11091(48) | 0.04335(17) | 0.615(12) | 1.48 | 0.00015 | 0.011 | 7237.386776(100) | 2.89973797(38) | 8.0(9.6) |
| HD189733 | 106 | 27 + 32 | 12800 | 0.15703(32) | 0.037514(48) | 0.6646(20) | 2.10 | 0.00029 | 0.17 | 3968.837026(20) | 2.21857545(15) | −5.3(1.9) |
| Kelt-1 | 34 | 12 + 14 | 938 | 0.07584(82) | 0.05682(28) | 0.05(64) | 1.91 | 0.00092 | 0.023 | 8026.51487(14) | 1.21749220(71) | −20.6(8.6) |
| Qatar-2 | 59 | 12 + 20 | 1750 | 0.16165(91) | 0.03812(11) | 0.129(63) | 1.26 | 0.00021 | 0.014 | 6045.458848(35) | 1.33711643(26) | 4.8(3.6) |
| TrES-1 | 56 | 13 + 23 | 1370 | 0.13799(83) | 0.05233(17) | 0.238(45) | 1.17 | 0.00029 | 0.0067 | 4350.354597(84) | 3.03006957(34) | 1.0(7.1) |
| WASP-2 | 68 | 20 + 19 | 1530 | 0.13315(50) | 0.03727(15) | 0.7382(50) | 1.47 | 0.00024 | 0.0042 | 5513.13577(12) | 2.15222222(39) | 3.0(8.0) |
| WASP-3 | 69 | 17 + 20 | 1710 | 0.10637(58) | 0.05700(18) | 0.492(17) | 1.53 | 0.00025 | 0.068 | 5325.825419(88) | 1.84683507(26) | 5.4(4.0) |
| WASP-4 | 66 | 22 + 22 | 4250 | 0.15488(32) | 0.044907(53) | 0.130(29) | 1.31 | 0.00019 | 0.0094 | 5045.738470(22) | 1.338231531(83) | −0.98(94) |
| WASP-5 | 17 | 9 + 3 | 1220 | 0.11459(79) | 0.05030(22) | 0.453(25) | 1.62 | 0.002 | 0.022 | 5896.57891(15) | 1.62843035(71) | −10(17) |
| WASP-6 | 18 | 8 + 3 | 1460 | 0.14310(88) | 0.05368(19) | 0.222(50) | 1.68 | 0.006 | 0.68 | 5379.546164(80) | 3.36100260(57) | −28(22) |
| WASP-12 | 230 | 84 + 72 | 9070 | 0.11840(17) | 0.062362(49) | 0.4312(48) | 1.35 | 0.00013 | 0.018 | 5994.401004(25) | 1.091420405(51) | −9.51(64) |
| WASP-52 | 72 | 25 + 20 | 2010 | 0.16538(51) | 0.03875(11) | 0.5985(62) | 1.56 | 0.00063 | 0.1 | 6904.792855(60) | 1.74978179(37) | −19(11) |
| XO-2N | 73 | 29 + 20 | 3930 | 0.10348(38) | 0.055937(92) | 0.194(40) | 1.44 | 0.0004 | 0.054 | 5167.935634(40) | 2.61585965(16) | −4.1(4.1) |
| XO-5 | 28 | 9 + 4 | 678 | 0.1026(15) | 0.06354(58) | 0.537(40) | 2.12 | 0.00075 | 0.01 | 7760.49334(36) | 4.1877641(22) | 258(67) |
| Corot-2 | 25 | 10 + 9 | 856 | 0.16557(99) | 0.04728(22) | 0.190(63) | 1.55 | 0.00061 | 0.0074 | 7629.40868(12) | 1.74299768(47) | 3.2(6.5) |
| GJ436[4] | 11 | 2 + 0 | 757 | 0.0829(15) | 0.02107(26) | 0.8664(78) | 1.32 | 0.041 | 0.66 | 4280.78227(12) | 2.6439052(85) | −160(190) |
| HAT-P-13 | 38 | 16 + 10 | 1420 | 0.08757(81) | 0.06895(39) | 0.7456(82) | 1.54 | 0.0015 | 0.037 | 5511.90699(19) | 2.9162394(14) | 96(34) |
| HAT-P-3 | 34 | 7 + 7 | 1340 | 0.11075(50) | 0.04337(18) | 0.622(12) | 1.54 | 0.00034 | 0.012 | 7237.38674(10) | 2.89973825(42) | 14(11) |
| HD189733 | 75 | 24 + 19 | 12800 | 0.15696(33) | 0.037525(48) | 0.6645(20) | 2.39 | 0.00046 | 0.17 | 3968.837031(20) | 2.21857545(16) | −5.6(2.0) |
| Kelt-1 | 18 | 6 + 5 | 887 | 0.07523(89) | 0.05694(31) | 0.13(26) | 1.57 | 0.0018 | 0.019 | 8026.51487(15) | 1.21749273(88) | −14(11) |
| Qatar-2 | 25 | 8 + 10 | 1720 | 0.16159(93) | 0.03810(11) | 0.125(66) | 1.40 | 0.0005 | 0.014 | 6034.761900(36) | 1.33711631(33) | 4.0(5.6) |
| TrES-1 | 44 | 14 + 18 | 1340 | 0.13772(85) | 0.05228(17) | 0.235(47) | 1.13 | 0.00036 | 0.0071 | 4347.324507(86) | 3.03006949(35) | 4.2(7.4) |
| WASP-2 | 32 | 12 + 10 | 1450 | 0.13328(52) | 0.03730(16) | 0.7378(54) | 1.64 | 0.00037 | 0.0059 | 5405.52461(14) | 2.15222181(58) | 10(10) |
| WASP-3 | 45 | 10 + 16 | 1660 | 0.10630(60) | 0.05704(19) | 0.495(18) | 1.52 | 0.00046 | 0.071 | 5325.825409(91) | 1.84683487(28) | 8.2(4.2) |
| WASP-4 | 50 | 17 + 19 | 4240 | 0.15488(32) | 0.044915(53) | 0.134(28) | 1.22 | 0.00025 | 0.0093 | 5045.738469(23) | 1.338231514(85) | −1.0(1.0) |
| WASP-5 | 15 | 8 + 3 | 1220 | 0.11477(79) | 0.05037(23) | 0.459(25) | 1.71 | 0.0026 | 0.022 | 5896.57894(15) | 1.62843056(75) | −16(19) |
| WASP-6 | 17 | 8 + 3 | 1460 | 0.14308(88) | 0.05368(19) | 0.220(51) | 1.72 | 0.0067 | 0.68 | 5379.546159(80) | 3.36100249(57) | −30(22) |
| WASP-12 | 203 | 78 + 58 | 9090 | 0.11839(17) | 0.062367(49) | 0.4316(48) | 1.33 | 0.00015 | 0.018 | 6003.132366(25) | 1.091420385(52) | −9.40(65) |
| WASP-52 | 44 | 19 + 10 | 1970 | 0.16530(53) | 0.03877(12) | 0.5965(65) | 1.59 | 0.0013 | 0.11 | 6904.792887(62) | 1.74978159(40) | −14(12) |
| XO-2N | 54 | 24 + 14 | 3920 | 0.10358(38) | 0.055930(92) | 0.207(37) | 1.56 | 0.00069 | 0.054 | 5212.405250(40) | 2.61585963(16) | −2.5(4.3) |
| XO-5 | 12 | 3 + 0 | 595 | 0.1024(20) | 0.06400(76) | 0.560(48) | 2.70 | 0.0015 | 0.0094 | 7802.37086(43) | 4.1877642(29) | 272(99) |

The fitting uncertainties are given in parenthesis after each estimation, in the units of the last two figures.

[1]Defined as $\mathcal{Q}'_{\rm sum} = \sqrt{\sum_{i=1}^{N} Q_i'^2}$.

[2]The quadratic TTV ephemeris and the value of $\chi^2_{\rm TTV}$ do not include the Southworth et al. (2009a,b, 2010) DFOSC data, because they may be affected by clock errors.

[3]Number of lightcurves fitted with individual red noise term + number of lightcurves fitted with shared $\tau$.

[4]Orbital eccentricity of $\sim 0.15$ is not taken into account, see Table 3 for a self-consistent fit.

[5]The realistic uncertainty also depends on the observed TTV scatter $\chi^2_{\rm TTV}$, likely inspired by the star activity, see text.

**Table 2.** Self-consistent fits of transit and radial velocity data: general, stellar, and other non-planetary parameters.

| host star | lightcurves num. total/red-noised | RV subsets num. total/red-noised | rad. accel. $c_1$ [m/s/yr] | star radius $R_\star$ [$R_\odot$] | rotation vel. $v \sin i$ [m/s] | alignment $\lambda$ [°] | limb-darkening $A_{\rm RV}$ | $B_{\rm RV}$ | RM effect correction[1] dataset group | $\nu$ [m/s] | $\mu$ [m/s] |
|---|---|---|---|---|---|---|---|---|---|---|---|
| Corot-2 | $25/(12+9)$ | 6/0 | −74(11) | 0.925(19) | 8930(400) | 3.1(6.6) | 0.469(72) | 0.06(12) | $HARPS_6$ | 30(840) | 7500(1300) |
| Corot-2'[2] | $25/(12+10)$ | 1/1 | −0.5(3.1) | 0.885(29) | 8570(430) | 3.0(8.2) | 0.465(72) | 0.06(12) | $HARPS_1$ | −280(950) | 7900(1300) |
| GJ436 | $47/(8+8)$ | 10/5 | 0.02(11) | 0.4266(89) | 1800(1000) | 354.5(4.9) | 0.56(28) | 0.05(35) | $HARPS_2$ | −1500(500) | −3100(2200) |
| | | | | | | | | | $HARPSN_5$ | −620(330) | −3200(1900) |
| | | | | | | | | | $KECK_2$ | −1230(610) | −3600(2100) |
| | | | | | | | | | $SOPHIE_1$ | — | — |
| HAT-P-13 | $38/(16+13)$ | 2/0 | 17.2(1.0) | 1.691(25) | 2300(1100) | 359.5(5.5) | 0.00(41) | 0.68(37) | $KECK_2$ | 180(600) | −1400(2300) |
| HAT-P-13' | $38/(16+13)$ | 1/0 | 17.56(85) | 1.692(25) | 2600(1300) | 0.0(5.4) | 0.00(38) | 0.69(35) | $KECK_1$ | 10(660) | −1900(2700) |
| HD189733 | $75/(31+24)$ | 14/4 | −1.07(75) | 0.7583(31) | 2280(110) | 0.08(36) | 0.67(14) | −0.07(17) | $HARPS_5$ | −36(70) | 2420(190) |
| | | | | | | | | | $HARPSN_2$ | −80(100) | 2310(210) |
| | | | | | | | | | $KECK_3$ | −2310(360) | 1900(430) |
| | | | | | | | | | $SOPHIE_4$ | 6200(2700) | −3300(3000) |
| TrES-1 | $44/(14+18)$ | 3/1 | −1.9(1.4) | 0.819(13) | — | — | — | — | $HARPSN_1$, $KECK_1$, $SOPHIE_1$ | | |
| WASP-2 | $32/(16+8)$ | 5/0 | −3.9(1.8) | 0.8200(82) | 960(850) | 345(18) | 0.65(15) | −0.04(18) | $HARPS_2$ | 0(1600) | −3700(1700) |
| | | | | | | | | | $KECK_1$ | — | — |
| | | | | | | | | | $SOPHIE_2$ | 100(4100) | 3200(4300) |
| WASP-3 | $45/(11+19)$ | 1/0 | −7.9(2.7) | 1.337(28) | — | — | — | — | $KECK_1$ | | |
| WASP-4 | $50/(19+15)$ | 4/2 | −0.7(1.1) | 0.9029(43) | 1890(220) | 344(16) | 0.269(97) | 0.34(15) | $CORALIE_1$ | — | — |
| | | | | | | | | | $HARPS_2$ | −120(310) | 460(650) |
| | | | | | | | | | $KECK_1$ | — | — |
| WASP-4'[2] | $50/(19+15)$ | 3/2 | −0.8(1.2) | 0.9045(46) | 1890(220) | 343(16) | 0.269(97) | 0.34(15) | $CORALIE_1$ | — | — |
| | | | | | | | | | $HARPS_2$ | −120(300) | 450(640) |
| | | | | | | | | | $KECK_1$ | — | — |
| WASP-5 | $15/(9+3)$ | 2/1 | −0.03(78) | 1.127(16) | 2470(400) | 0.2(6.4) | 0.72(16) | −0.16(22) | $HARPS_2$ | −670(960) | 3900(1100) |
| WASP-6 | $17/(9+3)$ | 5/0 | −420(260) | 0.829(23) | 1620(130) | 352(11) | 0.45(19) | 0.41(30) | $HARPS_5$ | 380(240) | 890(400) |
| WASP-12 | $203/(85+57)$ | 9/0 | −5.4(2.0) | 1.657(12) | 600(1200) | 9(48) | 0.378(30) | 0.140(45) | $HARPSN_1$ | — | — |
| | | | | | | | | | $KECK_1$ | — | — |
| | | | | | | | | | $SOPHIE_7$ | −1300(2700) | 2100(1600) |
| WASP-12' | $203/(85+57)$ | 3/2 | −7.5(2.2) | 1.660(16) | 1300(1500) | 75(30) | 0.378(30) | 0.141(45) | $HARPSN_1$ | — | — |
| | | | | | | | | | $KECK_1$ | — | — |
| | | | | | | | | | $SOPHIE_7$ | −3500(8400) | −100(3300) |
| XO-2N | $54/(25+17)$ | 3/1 | −1.2(1.2) | 0.986(14) | — | — | — | — | $HARPSN_1$, $KECK_1$, $SOPHIE_1$ | | |
| XO-5 | $12/(3+3)$ | 1/1 | 1.3(1.2) | 1.068(51) | — | — | — | — | $KECK_1$ | | |

The fitting uncertainties are given in parenthesis after each estimation, in the units of the last few figures. The star masses were assumed constant here (see the main paper), and their uncertainties were not included in the fit. Using the full set of transits for GJ436, while only the HQ (Stage 5) transits for other targets.

[1] Correction coefficients of the RM effect (Baluev & Shaidulin 2015). The index near the instrument name (e.g. $HARPS_6$) designates that the RV data for this instrument were splitted into that specified number of independent subsets (e.g. 5 short in-transit runs and yet another separate out-of-transit subset).

[2] A stroke stands for an alternative fit computed without splitting the RV data belonging to the same instrument.

**Table 3.** Self-consistent fits of transit and radial velocity data: planetary parameters.

| host star | planet mass $m_{\rm pl}$ $[M_{\rm Jup}]$ | planet radius $r_{\rm pl}$ $[R_{\rm Jup}]$ | orbital period[1] $P$ [d] | TTV trend[1,2,3] $T_{\rm d}$ [Myr] | mean longitude[1] $l$ [°] | inclination $i$ [°] | eccentricity $e$ | pericenter arg. $\omega$ [°] | $e\cos\omega$ | $e\sin\omega$ |
|---|---|---|---|---|---|---|---|---|---|---|
| Corot-2 | 2.744(51) | 1.523(36) | 1.74299686(44) | −11.2(9.4) | 359.4(1.6) | 88.15(56) | 0.042(18) | 60(18) | 0.021(14) | 0.037(17) |
| Corot-2’ | 2.85(10) | 1.455(51) | 1.74299682(45) | −10.4(8.2) | 0.7(2.4) | 88.32(52) | 0.013(26) | 320(130) | 0.009(21) | −0.008(32) |
| GJ436 | 0.06896(56) | 0.3581(97) | 2.64389856(36) | 7.1(3.2) | 335.82(44) | 86.83(10) | 0.1666(57) | 324.9(2.4) | 0.1363(34) | −0.0958(84) |
| HAT-P-13 b | 0.8528(59) | 1.465(30) | 2.9162384(17) | −2.42(86) | 158.64(41) | 82.12(22) | 0.0126(46) | 219(29) | −0.0098(35) | −0.0079(69) |
| c | 14.17(28) | — | 446.32(24) | — | 63.99(18) | — | 0.6621(58) | 175.28(37) | −0.6598(60) | 0.0545(39) |
| HAT-P-13’ b | 0.8532(53) | 1.466(30) | 2.9162383(17) | −2.41(85) | 158.58(35) | 82.10(22) | 0.0117(41) | 218(28) | −0.0092(30) | −0.0072(63) |
| c | 14.16(25) | — | 446.29(21) | — | 63.99(16) | — | 0.6614(50) | 175.28(32) | −0.6591(52) | 0.0545(35) |
| HD189733 | 1.1542(74) | 1.1840(52) | 2.218575123(57) | 28(12) | 20.45(38) | 85.712(36) | 0.0028(38) | 62(64) | 0.0013(33) | 0.0025(36) |
| TrES-1 | 0.6967(82) | 1.122(22) | 3.03006960(18) | −5.7(9.5) | 298.67(49) | 88.69(28) | 0.003(12) | 263(86) | −0.0004(43) | −0.003(12) |
| WASP-2 | 0.8711(73) | 1.087(14) | 2.15222163(67) | −12(11) | 214.37(25) | 84.82(10) | 0.0134(56) | 253(11) | −0.0039(21) | −0.0129(58) |
| WASP-3 | 1.982(49) | 1.419(32) | 1.84683480(30) | −11.1(5.5) | 274.88(83) | 84.24(32) | 0.010(15) | 41(74) | 0.0077(72) | 0.007(19) |
| WASP-4 | 1.1949(65) | 1.3915(82) | 1.338231501(75) | 47(45) | 235.80(26) | 88.63(30) | 0.0068(35) | 258(20) | −0.0015(22) | −0.0067(37) |
| WASP-4’ | 1.1976(68) | 1.3940(86) | 1.338231501(75) | 47(45) | 235.87(26) | 88.63(30) | 0.0053(38) | 247(28) | −0.0021(22) | −0.0049(41) |
| WASP-5 | 1.5351(80) | 1.294(25) | 1.6284311(14) | 5.2(6.3) | 343.01(32) | 84.57(33) | 0.0086(46) | 66(22) | 0.0035(30) | 0.0078(48) |
| WASP-6 | 0.458(20) | 1.175(35) | 3.36100264(65) | 14(14) | 32.6(2.4) | 89.00(36) | 0.036(24) | 116(36) | −0.016(21) | 0.033(26) |
| WASP-12 | 1.422(14) | 1.953(15) | 1.091421080(96) | 3.46(24) | 37.00(51) | 81.86(16) | 0.0259(74) | 250(11) | −0.0089(44) | −0.0243(77) |
| WASP-12’ | 1.413(15) | 1.956(20) | 1.091421078(96) | 3.47(24) | 36.82(49) | 81.96(18) | 0.024(11) | 252(11) | −0.0073(42) | −0.023(11) |
| XO-2N | 0.5924(68) | 1.017(16) | 2.61585963(16) | 80(140) | 198.72(48) | 88.33(25) | 0.008(13) | 91(29) | −0.0001(41) | 0.008(13) |
| XO-5 | 1.050(15) | 1.061(67) | 4.1877477(38) | −1.82(68) | 83.5(1.2) | 86.82(51) | 0.009(12) | 200(94) | −0.008(10) | −0.003(15) |

Same comments as in Table 2 also apply here.
[1]These parameters refer to $T_0 = 2455197.5$ (1 Jan, 2015) in the BJD TDB system.
[2]Except for WASP-12 case, the uncertainties for $T_{\rm d}$ are rather formal here, because this parameter becomes very nonlinear and nongaussian whenever it is comparable to the uncertainty. The linear parameter is $q = 1/T_{\rm d} = -\dot{P}/P$ with the uncertainty $\sigma_q = \sigma_{T_{\rm d}}/T_{\rm d}^2$.
[3]The realistic uncertainty in $T_{\rm d}$ also depends on the observed TTV scatter $\chi^2_{\rm TTV}$ from Table 1, see the main paper.

## REFERENCES


Baluev R. V., 2008, MNRAS, 385, 1279
Baluev R. V., Shaidulin V. S., 2015, MNRAS, 454, 4379
Bouma L. G., et al., 2019, AJ, 157, 217
Claret A., 2000, A&A, 363, 1081
Claret A., 2004, A&A, 428, 1001
Claret A., Bloemen S., 2011, A&A, 529, A75
Huitson C. M., Désert J.-M., Bean J. L., Fortney J. J., Stevenson K. B., Bergmann M., 2017, AJ, 154, 95
Patra K. C., Winn J. N., Holman M. J., Yu L., Deming D., Dai F., 2017, AJ, 154, 4
Southworth J., et al., 2009a, MNRAS, 396, 1023
Southworth J., et al., 2009b, MNRAS, 399, 287
Southworth J., et al., 2010, MNRAS, 408, 1680


This paper has been typeset from a TEX/LATEX file prepared by the author.
